# Supplementary material for: A Community-Driven Validation Service for Standard Medical Imaging Objects
Source: arXiv:1806.08987 source file (2018-06-26)
Supplement: Supplementary file 1 [file Suplementary.tex]

\documentclass[final,5p,times,twocolumn]{elsarticle}
\usepackage{lineno}
\usepackage{listings}
\usepackage{adjustbox}
\usepackage{caption} 
\usepackage{hyperref}
\modulolinenumbers[5]
\usepackage{graphicx}
\usepackage{amssymb}

\begin{document}

\begin{center}
\label{lst:xml1} 
\begin{adjustbox}{keepaspectratio,caption=Example of a validation JSON file}
\begin{lstlisting}[showstringspaces=false,caption=JSON file produced from the results of the validation of the Computed Radiography Image mentioned in Section \ref{S:5}]
{"messagetype":"result","validationid":"8r5vl6hcsm0ljoendga4jfiqud","date":"2017-08-02 18:36:49","service":"Computed Radiography Image Storage",,"valid":false,"results":[{"ie":"Patient","module":"Patient","status":"WARNING","inconsistencies":{"missing_attributes":[{"tag":"(0010,0200)","type":"TYPE_3","keyword":"QualityControlSubject","vr":"CS"},{"tag":"(0008,1120)","type":"TYPE_3","keyword":"ReferencedPatientSequence","vr":"SQ"},{"tag":"(0010,0032)","type":"TYPE_3","keyword":"PatientBirthTime","vr":"TM"},{"tag":"(0010,1000)","type":"TYPE_3","keyword":"OtherPatientIDs","vr":"LO"},{"tag":"(0010,1002)","type":"TYPE_3","keyword":"OtherPatientIDsSequence","vr":"SQ"},{"tag":"(0010,1001)","type":"TYPE_3","keyword":"OtherPatientNames","vr":"PN"},{"tag":"(0010,2160)","type":"TYPE_3","keyword":"EthnicGroup","vr":"SH"},{"tag":"(0010,4000)","type":"TYPE_3","keyword":"PatientComments","vr":"LT"},{"tag":"(0012,0062)","type":"TYPE_3","keyword":"PatientIdentityRemoved","vr":"CS"}],"missing_values":[],"invalid_values":[],"not_allowed":[]}},{"ie":"Patient","module":"ClinicalTrialSubject","status":"HAS ERRORS","inconsistencies":{"missing_attributes":[{"tag":"(0012,0010)","type":"TYPE_1","keyword":"ClinicalTrialSponsorName","vr":"LO"},{"tag":"(0012,0020)","type":"TYPE_1","keyword":"ClinicalTrialProtocolID","vr":"LO"},{"tag":"(0012,0021)","type":"TYPE_2","keyword":"ClinicalTrialProtocolName","vr":"LO"},{"tag":"(0012,0030)","type":"TYPE_2","keyword":"ClinicalTrialSiteID","vr":"LO"},{"tag":"(0012,0031)","type":"TYPE_2","keyword":"ClinicalTrialSiteName","vr":"LO"},{"tag":"(0012,0040)","type":"TYPE_1C","keyword":"ClinicalTrialSubjectID","vr":"LO"},{"tag":"(0012,0042)","type":"TYPE_1C","keyword":"ClinicalTrialSubjectReadingID","vr":"LO"},{"tag":"(0012,0082)","type":"TYPE_3","keyword":"ClinicalTrialProtocolEthicsCommitteeApprovalNumber","vr":"LO"}],"missing_values":[],"invalid_values":[],"not_allowed":[]}},{"ie":"Study","module":"GeneralStudy","status":"WARNING","inconsistencies":{"missing_attributes":[{"tag":"(0008,0096)","type":"TYPE_3","keyword":"ReferringPhysicianIdentificationSequence","vr":"SQ"},{"tag":"(0008,0051)","type":"TYPE_3","keyword":"IssuerOfAccessionNumberSequence","vr":"SQ"},{"tag":"(0008,1048)","type":"TYPE_3","keyword":"PhysiciansOfRecord","vr":"PN"},{"tag":"(0008,1049)","type":"TYPE_3","keyword":"PhysiciansOfRecordIdentificationSequence","vr":"SQ"},{"tag":"(0008,1062)","type":"TYPE_3","keyword":"PhysiciansReadingStudyIdentificationSequence","vr":"SQ"},{"tag":"(0032,1034)","type":"TYPE_3","keyword":"RequestingServiceCodeSequence","vr":"SQ"},{"tag":"(0008,1110)","type":"TYPE_3","keyword":"ReferencedStudySequence","vr":"SQ"},{"tag":"(0008,1032)","type":"TYPE_3","keyword":"ProcedureCodeSequence","vr":"SQ"},{"tag":"(0040,1012)","type":"TYPE_3","keyword":"ReasonForPerformedProcedureCodeSequence","vr":"SQ"}],"missing_values":[],"invalid_values":[],"not_allowed":[]}},{"ie":"Study","module":"PatientStudy","status":"WARNING","inconsistencies":{"missing_attributes":[{"tag":"(0008,1080)","type":"TYPE_3","keyword":"AdmittingDiagnosesDescription","vr":"LO"},{"tag":"(0008,1084)","type":"TYPE_3","keyword":"AdmittingDiagnosesCodeSequence","vr":"SQ"},{"tag":"(0010,1010)","type":"TYPE_3","keyword":"PatientAge","vr":"AS"},{"tag":"(0010,1020)","type":"TYPE_3","keyword":"PatientSize","vr":"DS"},{"tag":"(0010,1030)","type":"TYPE_3","keyword":"PatientWeight","vr":"DS"},{"tag":"(0010,1021)","type":"TYPE_3","keyword":"PatientSizeCodeSequence","vr":"SQ"},{"tag":"(0010,2180)","type":"TYPE_3","keyword":"Occupation","vr":"SH"},{"tag":"(0010,21B0)","type":"TYPE_3","keyword":"AdditionalPatientHistory","vr":"LT"},{"tag":"(0038,0010)","type":"TYPE_3","keyword":"AdmissionID","vr":"LO"},{"tag":"(0038,0014)","type":"TYPE_3","keyword":"IssuerOfAdmissionIDSequence","vr":"SQ"},{"tag":"(0038,0060)","type":"TYPE_3","keyword":"ServiceEpisodeID","vr":"LO"},{"tag":"(0038,0064)","type":"TYPE_3","keyword":"IssuerOfServiceEpisodeIDSequence","vr":"SQ"},{"tag":"(0038,0062)","type":"TYPE_3","keyword":"ServiceEpisodeDescription","vr":"LO"}],"missing_values":[],"invalid_values":[],"not_allowed":[]}},{"ie":"Study","module":"ClinicalTrialStudy","status":"HAS ERRORS","inconsistencies":{"missing_attributes":[{"tag":"(0012,0050)","type":"TYPE_2","keyword":"ClinicalTrialTimePointID","vr":"LO"},{"tag":"(0012,0051)","type":"TYPE_3","keyword":"ClinicalTrialTimePointDescription","vr":"ST"},{"tag":"(0012,0083)","type":"TYPE_3","keyword":"ConsentForClinicalTrialUseSequence","vr":"SQ"}],"missing_values":[],"invalid_values":[],"not_allowed":[]}},{"ie":"Series","module":"GeneralSeries","status":"WARNING","inconsistencies":{"missing_attributes":[{"tag":"(0008,0021)","type":"TYPE_3","keyword":"SeriesDate","vr":"DA"},{"tag":"(0008,0031)","type":"TYPE_3","keyword":"SeriesTime","vr":"TM"},{"tag":"(0008,1050)","type":"TYPE_3","keyword":"PerformingPhysicianName","vr":"PN"},{"tag":"(0008,1052)","type":"TYPE_3","keyword":"PerformingPhysicianIdentificationSequence","vr":"SQ"},{"tag":"(0008,103F)","type":"TYPE_3","keyword":"SeriesDescriptionCodeSequence","vr":"SQ"},{"tag":"(0008,1070)","type":"TYPE_3","keyword":"OperatorsName","vr":"PN"},{"tag":"(0008,1072)","type":"TYPE_3","keyword":"OperatorIdentificationSequence","vr":"SQ"},{"tag":"(0008,1111)","type":"TYPE_3","keyword":"ReferencedPerformedProcedureStepSequence","vr":"SQ"},{"tag":"(0008,1250)","type":"TYPE_3","keyword":"RelatedSeriesSequence","vr":"SQ"},{"tag":"(0028,0108)","type":"TYPE_3","keyword":"SmallestPixelValueInSeries","vr":"SS"},{"tag":"(0028,0108)","type":"TYPE_3","keyword":"SmallestPixelValueInSeries","vr":"US"},{"tag":"(0028,0109)","type":"TYPE_3","keyword":"LargestPixelValueInSeries","vr":"SS"},{"tag":"(0028,0109)","type":"TYPE_3","keyword":"LargestPixelValueInSeries","vr":"US"},{"tag":"(0040,0275)","type":"TYPE_3","keyword":"RequestAttributesSequence","vr":"SQ"}],"missing_values":[],"invalid_values":[],"not_allowed":[]}},{"ie":"Series","module":"CRSeries","status":"HAS ERRORS","inconsistencies":{"missing_attributes":[{"tag":"(0018,1160)","type":"TYPE_2","keyword":"FilterType","vr":"SH"},{"tag":"(0018,1180)","type":"TYPE_3","keyword":"CollimatorGridName","vr":"SH"},{"tag":"(0018,1190)","type":"TYPE_3","keyword":"FocalSpots","vr":"DS"},{"tag":"(0018,1260)","type":"TYPE_3","keyword":"PlateType","vr":"DS"},{"tag":"(0018,1261)","type":"TYPE_3","keyword":"PhosphorType","vr":"LO"}],"missing_values":[],"invalid_values":[],"not_allowed":[]}},{"ie":"Series","module":"ClinicalTrialSeries","status":"HAS ERRORS","inconsistencies":{"missing_attributes":[{"tag":"(0012,0060)","type":"TYPE_2","keyword":"ClinicalTrialCoordinatingCenterName","vr":"LO"},{"tag":"(0012,0071)","type":"TYPE_3","keyword":"ClinicalTrialSeriesID","vr":"LO"},{"tag":"(0012,0072)","type":"TYPE_3","keyword":"ClinicalTrialSeriesDescription","vr":"LO"}],"missing_values":[],"invalid_values":[],"not_allowed":[]}},{"ie":"Equipment","module":"GeneralEquipment","status":"WARNING","inconsistencies":{"missing_attributes":[{"tag":"(0008,0081)","type":"TYPE_3","keyword":"InstitutionAddress","vr":"ST"},{"tag":"(0008,1010)","type":"TYPE_3","keyword":"StationName","vr":"SH"},{"tag":"(0008,1040)","type":"TYPE_3","keyword":"InstitutionalDepartmentName","vr":"LO"},{"tag":"(0018,1000)","type":"TYPE_3","keyword":"DeviceSerialNumber","vr":"LO"},{"tag":"(0008,1020)","type":"TYPE_3","keyword":"","vr":"LO"},{"tag":"(0018,1008)","type":"TYPE_3","keyword":"GantryID","vr":"LO"},{"tag":"(0018,1050)","type":"TYPE_3","keyword":"SpatialResolution","vr":"DS"},{"tag":"(0018,1200)","type":"TYPE_3","keyword":"DateOfLastCalibration","vr":"DA"},{"tag":"(0018,1201)","type":"TYPE_3","keyword":"TimeOfLastCalibration","vr":"TM"}],"missing_values":[],"invalid_values":[],"not_allowed":[]}},{"ie":"Image","module":"GeneralImage","status":"HAS ERRORS","inconsistencies":{"missing_attributes":[{"tag":"(0020,0020)","type":"TYPE_1C","keyword":"PatientOrientation","vr":"CS"},{"tag":"(0008,0023)","type":"TYPE_2C","keyword":"ContentDate","vr":"DA"},{"tag":"(0008,0033)","type":"TYPE_2C","keyword":"ContentTime","vr":"TM"},{"tag":"(0008,0008)","type":"TYPE_3","keyword":"ImageType","vr":"CS"},{"tag":"(0020,0012)","type":"TYPE_3","keyword":"AcquisitionNumber","vr":"IS"},{"tag":"(0008,0022)","type":"TYPE_3","keyword":"AcquisitionDate","vr":"DA"},{"tag":"(0008,0032)","type":"TYPE_3","keyword":"AcquisitionTime","vr":"TM"},{"tag":"(0008,002A)","type":"TYPE_3","keyword":"AcquisitionDateTime","vr":"DT"},{"tag":"(0008,1140)","type":"TYPE_3","keyword":"ReferencedImageSequence","vr":"SQ"},{"tag":"(0008,2111)","type":"TYPE_3","keyword":"DerivationDescription","vr":"ST"},{"tag":"(0008,9215)","type":"TYPE_3","keyword":"DerivationCodeSequence","vr":"SQ"},{"tag":"(0008,2112)","type":"TYPE_3","keyword":"SourceImageSequence","vr":"SQ"},{"tag":"(0008,114A)","type":"TYPE_3","keyword":"ReferencedInstanceSequence","vr":"SQ"},{"tag":"(0020,1002)","type":"TYPE_3","keyword":"ImagesInAcquisition","vr":"IS"},{"tag":"(0020,4000)","type":"TYPE_3","keyword":"ImageComments","vr":"LT"},{"tag":"(0028,0300)","type":"TYPE_3","keyword":"QualityControlImage","vr":"CS"},{"tag":"(0028,0301)","type":"TYPE_3","keyword":"BurnedInAnnotation","vr":"CS"},{"tag":"(0028,0302)","type":"TYPE_3","keyword":"RecognizableVisualFeatures","vr":"CS"},{"tag":"(0028,2110)","type":"TYPE_3","keyword":"LossyImageCompression","vr":"CS"},{"tag":"(0028,2112)","type":"TYPE_3","keyword":"LossyImageCompressionRatio","vr":"DS"},{"tag":"(0028,2114)","type":"TYPE_3","keyword":"LossyImageCompressionMethod","vr":"CS"},{"tag":"(0088,0200)","type":"TYPE_3","keyword":"IconImageSequence","vr":"SQ"},{"tag":"(2050,0020)","type":"TYPE_3","keyword":"PresentationLUTShape","vr":"CS"},{"tag":"(0008,3010)","type":"TYPE_3","keyword":"IrradiationEventUID","vr":"UI"},{"tag":"(0040,9096)","type":"TYPE_3","keyword":"RealWorldValueMappingSequence","vr":"SQ"}],"missing_values":[],"invalid_values":[],"not_allowed":[]}},{"ie":"Image","module":"ImagePixel","status":"HAS ERRORS","inconsistencies":{"missing_attributes":[{"tag":"(0028,7FE0)","type":"TYPE_1C","keyword":"PixelDataProviderURL","vr":"UT"},{"tag":"(0028,0121)","type":"TYPE_3","keyword":"PixelPaddingRangeLimit","vr":"US"},{"tag":"(0028,0121)","type":"TYPE_3","keyword":"PixelPaddingRangeLimit","vr":"SS"}],"missing_values":[],"invalid_values":[],"not_allowed":[]}},{"ie":"Image","module":"ContrastBolus","status":"HAS ERRORS","inconsistencies":{"missing_attributes":[{"tag":"(0018,0010)","type":"TYPE_2","keyword":"ContrastBolusAgent","vr":"LO"},{"tag":"(0018,0012)","type":"TYPE_3","keyword":"ContrastBolusAgentSequence","vr":"SQ"},{"tag":"(0018,1040)","type":"TYPE_3","keyword":"ContrastBolusRoute","vr":"LO"},{"tag":"(0018,0014)","type":"TYPE_3","keyword":"ContrastBolusAdministrationRouteSequence","vr":"SQ"},{"tag":"(0018,1041)","type":"TYPE_3","keyword":"ContrastBolusVolume","vr":"DS"},{"tag":"(0018,1042)","type":"TYPE_3","keyword":"ContrastBolusStartTime","vr":"TM"},{"tag":"(0018,1043)","type":"TYPE_3","keyword":"ContrastBolusStopTime","vr":"TM"},{"tag":"(0018,1044)","type":"TYPE_3","keyword":"ContrastBolusTotalDose","vr":"DS"},{"tag":"(0018,1046)","type":"TYPE_3","keyword":"ContrastFlowRate","vr":"DS"},{"tag":"(0018,1047)","type":"TYPE_3","keyword":"ContrastFlowDuration","vr":"DS"},{"tag":"(0018,1048)","type":"TYPE_3","keyword":"ContrastBolusIngredient","vr":"DS"},{"tag":"(0018,1049)","type":"TYPE_3","keyword":"ContrastBolusIngredientConcentration","vr":"DS"}],"missing_values":[],"invalid_values":[],"not_allowed":[]}},{"ie":"Image","module":"DisplayShutter","status":"HAS ERRORS","inconsistencies":{"missing_attributes":[{"tag":"(0018,1600)","type":"TYPE_1","keyword":"ShutterShape","vr":"CS"},{"tag":"(0018,1622)","type":"TYPE_3","keyword":"ShutterPresentationValue","vr":"US"},{"tag":"(0018,1624)","type":"TYPE_3","keyword":"ShutterPresentationColorCIELabValue","vr":"US"}],"missing_values":[],"invalid_values":[],"not_allowed":[]}},{"ie":"Image","module":"Device","status":"HAS ERRORS","inconsistencies":{"missing_attributes":[{"tag":"(0050,0010)","type":"TYPE_1","keyword":"DeviceSequence","vr":"SQ"}],"missing_values":[],"invalid_values":[],"not_allowed":[]}},{"ie":"Image","module":"Specimen","status":"HAS ERRORS","inconsistencies":{"missing_attributes":[{"tag":"(0040,0512)","type":"TYPE_1","keyword":"ContainerIdentifier","vr":"LO"},{"tag":"(0040,0513)","type":"TYPE_2","keyword":"IssuerOfTheContainerIdentifierSequence","vr":"SQ"},{"tag":"(0040,0515)","type":"TYPE_3","keyword":"AlternateContainerIdentifierSequence","vr":"SQ"},{"tag":"(0040,0518)","type":"TYPE_2","keyword":"ContainerTypeCodeSequence","vr":"SQ"},{"tag":"(0040,051A)","type":"TYPE_3","keyword":"ContainerDescription","vr":"LO"},{"tag":"(0040,0520)","type":"TYPE_3","keyword":"ContainerComponentSequence","vr":"SQ"},{"tag":"(0040,0560)","type":"TYPE_1","keyword":"SpecimenDescriptionSequence","vr":"SQ"}],"missing_values":[],"invalid_values":[],"not_allowed":[]}},{"ie":"Image","module":"CRImage","status":"WARNING","inconsistencies":{"missing_attributes":[{"tag":"(0018,0060)","type":"TYPE_3","keyword":"KVP","vr":"DS"},{"tag":"(0018,1110)","type":"TYPE_3","keyword":"DistanceSourceToDetector","vr":"DS"},{"tag":"(0018,1111)","type":"TYPE_3","keyword":"DistanceSourceToPatient","vr":"DS"},{"tag":"(0018,1150)","type":"TYPE_3","keyword":"ExposureTime","vr":"FD"},{"tag":"(0018,1151)","type":"TYPE_3","keyword":"XRayTubeCurrent","vr":"IS"},{"tag":"(0018,1152)","type":"TYPE_3","keyword":"Exposure","vr":"IS"},{"tag":"(0018,1153)","type":"TYPE_3","keyword":"ExposureInuAs","vr":"IS"},{"tag":"(0018,1164)","type":"TYPE_3","keyword":"ImagerPixelSpacing","vr":"DS"},{"tag":"(0018,1170)","type":"TYPE_3","keyword":"GeneratorPower","vr":"IS"},{"tag":"(0018,1400)","type":"TYPE_3","keyword":"AcquisitionDeviceProcessingDescription","vr":"LO"},{"tag":"(0018,1401)","type":"TYPE_3","keyword":"AcquisitionDeviceProcessingCode","vr":"LO"},{"tag":"(0018,1402)","type":"TYPE_3","keyword":"CassetteOrientation","vr":"CS"},{"tag":"(0018,1403)","type":"TYPE_3","keyword":"CassetteSize","vr":"CS"},{"tag":"(0018,1404)","type":"TYPE_3","keyword":"ExposuresOnPlate","vr":"US"},{"tag":"(0018,1600)","type":"TYPE_3","keyword":"ShutterShape","vr":"DS"}],"missing_values":[],"invalid_values":[],"not_allowed":[]}},{"ie":"Image","module":"OverlayPlane","status":"HAS ERRORS","inconsistencies":{"missing_attributes":[{"tag":"(6000,0010)","type":"TYPE_1","keyword":"OverlayRows","vr":"US"},{"tag":"(6000,0011)","type":"TYPE_1","keyword":"OverlayColumns","vr":"US"},{"tag":"(6000,0040)","type":"TYPE_1","keyword":"OverlayType","vr":"CS"},{"tag":"(6000,0050)","type":"TYPE_1","keyword":"OverlayOrigin","vr":"SS"},{"tag":"(6000,0100)","type":"TYPE_1","keyword":"OverlayBitsAllocated","vr":"US"},{"tag":"(6000,0102)","type":"TYPE_1","keyword":"OverlayBitPosition","vr":"US"},{"tag":"(6000,3000)","type":"TYPE_1","keyword":"OverlayData","vr":"OB"},{"tag":"(6000,3000)","type":"TYPE_1","keyword":"OverlayData","vr":"OW"},{"tag":"(6000,0022)","type":"TYPE_3","keyword":"OverlayDescription","vr":"LO"},{"tag":"(6000,0045)","type":"TYPE_3","keyword":"OverlaySubtype","vr":"LO"},{"tag":"(6000,1500)","type":"TYPE_3","keyword":"OverlayLabel","vr":"LO"},{"tag":"(6000,1301)","type":"TYPE_3","keyword":"ROIArea","vr":"IS"},{"tag":"(6000,1302)","type":"TYPE_3","keyword":"ROIMean","vr":"DS"},{"tag":"(6000,1303)","type":"TYPE_3","keyword":"ROIStandardDeviation","vr":"DS"}],"missing_values":[],"invalid_values":[],"not_allowed":[]}},{"ie":"Image","module":"ModalityLUT","status":"VALID","inconsistencies":{}},{"ie":"Image","module":"VOILUT","status":"WARNING","inconsistencies":{"missing_attributes":[{"tag":"(0028,1055)","type":"TYPE_3","keyword":"WindowCenterWidthExplanation","vr":"LO"},{"tag":"(0028,1056)","type":"TYPE_3","keyword":"VOILUTFunction","vr":"CS"}],"missing_values":[],"invalid_values":[],"not_allowed":[]}},{"ie":"Image","module":"SOPCommon","status":"HAS ERRORS","inconsistencies":{"missing_attributes":[{"tag":"(0008,0012)","type":"TYPE_3","keyword":"InstanceCreationDate","vr":"DA"},{"tag":"(0008,0013)","type":"TYPE_3","keyword":"InstanceCreationTime","vr":"TM"},{"tag":"(0008,0015)","type":"TYPE_3","keyword":"InstanceCoercionDateTime","vr":"DT"},{"tag":"(0008,0014)","type":"TYPE_3","keyword":"InstanceCreatorUID","vr":"UI"},{"tag":"(0008,001A)","type":"TYPE_3","keyword":"RelatedGeneralSOPClassUID","vr":"UI"},{"tag":"(0008,001B)","type":"TYPE_3","keyword":"OriginalSpecializedSOPClassUID","vr":"UI"},{"tag":"(0008,0110)","type":"TYPE_3","keyword":"CodingSchemeIdentificationSequence","vr":"SQ"},{"tag":"(0008,0201)","type":"TYPE_3","keyword":"TimezoneOffsetFromUTC","vr":"SH"},{"tag":"(0018,A001)","type":"TYPE_3","keyword":"ContributingEquipmentSequence","vr":"SQ"},{"tag":"(0100,0410)","type":"TYPE_3","keyword":"SOPInstanceStatus","vr":"CS"},{"tag":"(0100,0420)","type":"TYPE_3","keyword":"SOPAuthorizationDateTime","vr":"DT"},{"tag":"(0100,0424)","type":"TYPE_3","keyword":"SOPAuthorizationComment","vr":"LT"},{"tag":"(0100,0426)","type":"TYPE_3","keyword":"AuthorizationEquipmentCertificationNumber","vr":"LO"},{"tag":"(0400,0500)","type":"TYPE_1C","keyword":"EncryptedAttributesSequence","vr":"SQ"},{"tag":"(0400,0561)","type":"TYPE_3","keyword":"OriginalAttributesSequence","vr":"SQ"},{"tag":"(0028,0303)","type":"TYPE_3","keyword":"LongitudinalTemporalInformationModified","vr":"CS"},{"tag":"(0008,0053)","type":"TYPE_1C","keyword":"QueryRetrieveView","vr":"CS"},{"tag":"(0020,9172)","type":"TYPE_1C","keyword":"ConversionSourceAttributesSequence","vr":"SQ"}],"missing_values":[],"invalid_values":[],"not_allowed":[]}},{"ie":"Image","module":"CommonInstanceReference","status":"HAS ERRORS","inconsistencies":{"missing_attributes":[{"tag":"(0008,1115)","type":"TYPE_1C","keyword":"ReferencedSeriesSequence","vr":"SQ"},{"tag":"(0008,1200)","type":"TYPE_1","keyword":"StudiesContainingOtherReferencedInstancesSequence","vr":"SQ"}],"missing_values":[],"invalid_values":[],"not_allowed":[]}}]}
\end{lstlisting}
\end{adjustbox}
\end{center}

\end{document}
